# Supplementary material for: Multi-Modal Forecaster: Jointly Predicting Time Series and Textual Data
Source: arXiv:2411.06735 source file (2024-11-21)
Supplement: Supplementary file 1 [file B_appendix.tex]

\section{All Models and Metrics}\label{app:models_metrics}

This section includes all the numerical results for our experiments. As noted above,
the same set of experiments were conducted across all three of our datasets. 
% Note that there are some missing values, which are currently still being processed.

The models we evaluated include the following. 
\begin{enumerate}
    \item Input\_Copy: A baseline model that simply copies the input as the output, used to establish a performance floor. We use this model in both
    the text and time modalities.
    
    \item NLinear: A simple linear projection time series forecasting model proposed by \citep{zeng2022transformers}
    
    \item Linear\_Text\_Embedding: We extend the capabilities
    of the NLinear model by introducing text embeddings as covariates. We use
    the \textit{bge-small-en-v1.5} text embedding model to accomplish this.

    \item Text2Text: Language models 
    prompted with textual events, forecasting textual events only. We evaluate the different capabilities
    of zero-shot, in-context, and fine-tuned models. 

    \item TextTime2Text: Language models take both text and time data as input but only forecast textual events. We convert time-series data to text and combine it with the textual input. We evaluate the different capabilities
    of zero-shot, in-context, and fine-tuned models. 

    \item TextTime2Time: Language models process both textual and time-series inputs but predict only future time-series data. Textual inputs provide context for numerical forecasts. We evaluate the different capabilities
    of zero-shot, in-context, and fine-tuned models. 
    
    \item TextTime2TextTime: Language models provided with both both text and time data. The numerical time-series data 
    is stringified and concatenated to the text. We prompt the model to predict either text or time. 
    We evaluate the different capabilities
    of zero-shot, in-context, and fine-tuned models. 
    
    \item PatchTST: A Patch-based Time Series Transformer model for forecasting,
    proposed by \citep{nie2022time}.
    
    \item Hybrid: Our hybrid model, with details presented in Figure \ref{fig:hybrid_model}.
\end{enumerate}
